# Supplementary material for: SuperGS: Super-Resolution 3D Gaussian Splatting Enhanced by Variational Residual Features and Uncertainty-Augmented Learning
Source: arXiv:2410.02571 source file (2024-12-11)
Supplement: Supplementary file 1 [file supplementary.tex]

\clearpage
\setcounter{page}{1}
\setcounter{section}{0}
\maketitlesupplementary

\section{Additional Results}
\label{sec:rationale}
In this section, we present comprehensive quantitative evaluations on both real-world~\cite{barron2022mip, hedman2018deep, knapitsch2017tanks} and synthetic~\cite{mildenhall2021nerf} datasets. The performance is measured using three standard metrics: PSNR, SSIM, and LPIPS, as detailed in Table~\ref{realworld-psnrx4}.

\begin{table*}[!ht]
        \footnotesize
        \centering
        \caption{PSNR scores for Real-world Datasets on HRNVS ($\times4$) task.}
        \label{tab:realworld-psnrx4}
    \begin{tabular}{L{2.2cm}|C{0.75cm}C{0.75cm}C{0.75cm}C{0.75cm}C{0.75cm}C{0.75cm}C{0.75cm}C{0.75cm}C{0.75cm}|C{1.1cm}C{1.1cm}|C{0.75cm}C{0.75cm}} % {c|ccc|ccc|ccc}
\toprule
Dataset     & \multicolumn{9}{c|}{Mip-NeRF360} & \multicolumn{2}{c|}{Tanks\&Temples} & \multicolumn{2}{c}{Deep Blending}   \\
Methods\&Scenes     &room   &kitchen  &bonsai &counter   &bicycle &flowers &garden   &stump &treehill &drjohnson  &playroom  &train &truck\\ \midrule

3DGS            &26.01 &19.70 &22.77
                &23.24 &18.78 &17.69
                &18.33 &20.54 &19.42
                &26.35 &27.07 &18.67 &17.97 \\

3DGS-SwinIR     &30.46 &29.05 &30.42
                &28.08 &23.94 &20.87
                &24.47 &26.13 &21.95
                &27.89 &28.83 &19.77 &21.24 \\

GaussianSR      &30.58 &28.27 &30.23
                &28.02 &22.63 &20.61
                &23.72 &24.38 &21.98
                &27.81 &28.76 &- &- \\ 
                
SRGS            &31.09 &29.81 &31.28
                &28.63 &24.18 &20.86
                &25.01 &26.22 &22.26
                &28.90 &29.90 &19.88 &21.52 \\ \midrule

\textbf{Ours}   &\textbf{31.73} &\textbf{30.22} &\textbf{32.46}
                &\textbf{29.65} &\textbf{24.58} &\textbf{21.19}
                &\textbf{25.19} &\textbf{26.57} &\textbf{22.45}
                &\textbf{29.37} &\textbf{30.37} &\textbf{20.45} &\textbf{21.92} \\
\bottomrule
\end{tabular}
\end{table*}

\clearpage
